# Supplementary material for: Deep Retrieval: Learning A Retrievable Structure for Large-Scale Recommendations
Source: arXiv:2007.07203 source file (2021-05-18)
Supplement: Supplementary file 1 [file appendix.tex]

\subsection{Precision and F-measure against hyperparameters}

Here we plot the precision@200 and F-measure@200 against hyperparameters in the Amazon books datasets. The results of precision@200 are shown in Figure~\ref{fig:hyperparameters_2} and the results of F-measure@200 are shown in Figure~\ref{fig:hyperparameters_3}. We can see that both the precision and the F-measure follow the same trend as the recall shown in Section~\ref{sec:exp}.3.

%\begin{algorithm}[t]
%    \caption{Coordinate descent algorithm for penalized path assignment}
%   \label{alg:coodinate-descent}
%   \begin{algorithmic}
%      \STATE {\bfseries Input:} Score functions $\log s[v, c]$. Number of iterations $T$.
%      \STATE Initialize $|c| = 0$ for all paths $c$.
%      \FOR{$t=1$ {\bfseries to} $T$}
%        \FOR{all items $v$}
%            \STATE ${\rm sum} \leftarrow 0$.
%            \FOR{$j=1$ {\bfseries to} $J$}
%                \IF {$t > 1$}
%                    \STATE $|\pi^{(t-1)}_j(v)| \leftarrow |\pi^{(t-1)}_j(v)| - 1$.
%                \ENDIF
%                \FOR{all candidate paths $c$ of item $v$ such that $c \not\in \{\pi_l^{(t)}(v)\}_{l=1}^{j-1}$}
%                    \STATE Compute penalized scores $$\tilde{s}[v, c] = \log \left( s[v, c] + {\rm sum} \right) - \alpha \left( f(|c|+1) - f(|c|) \right).$$
%                \ENDFOR
%                \STATE $\pi_j^{(t)}(v) \leftarrow \arg\max_c \tilde{s}[v, c]$.
%                \STATE ${\rm sum} \leftarrow  {\rm sum} + s[v, \pi_j^{(t)}(v)]$.
%                \STATE $|\pi_j^{(t)}(v)| \leftarrow |\pi_j^{(t)}(v)| + 1$.
%            \ENDFOR
%        \ENDFOR
%   \ENDFOR
%   \STATE {\bfseries Output:} path assignments $\{\pi^{(T)}_j(v)\}_{j=1}^J$.
%   \end{algorithmic}
%\end{algorithm}

\newpage

% \begin{figure}[H]
%     \centering
%     \includegraphics[width=0.45\textwidth]{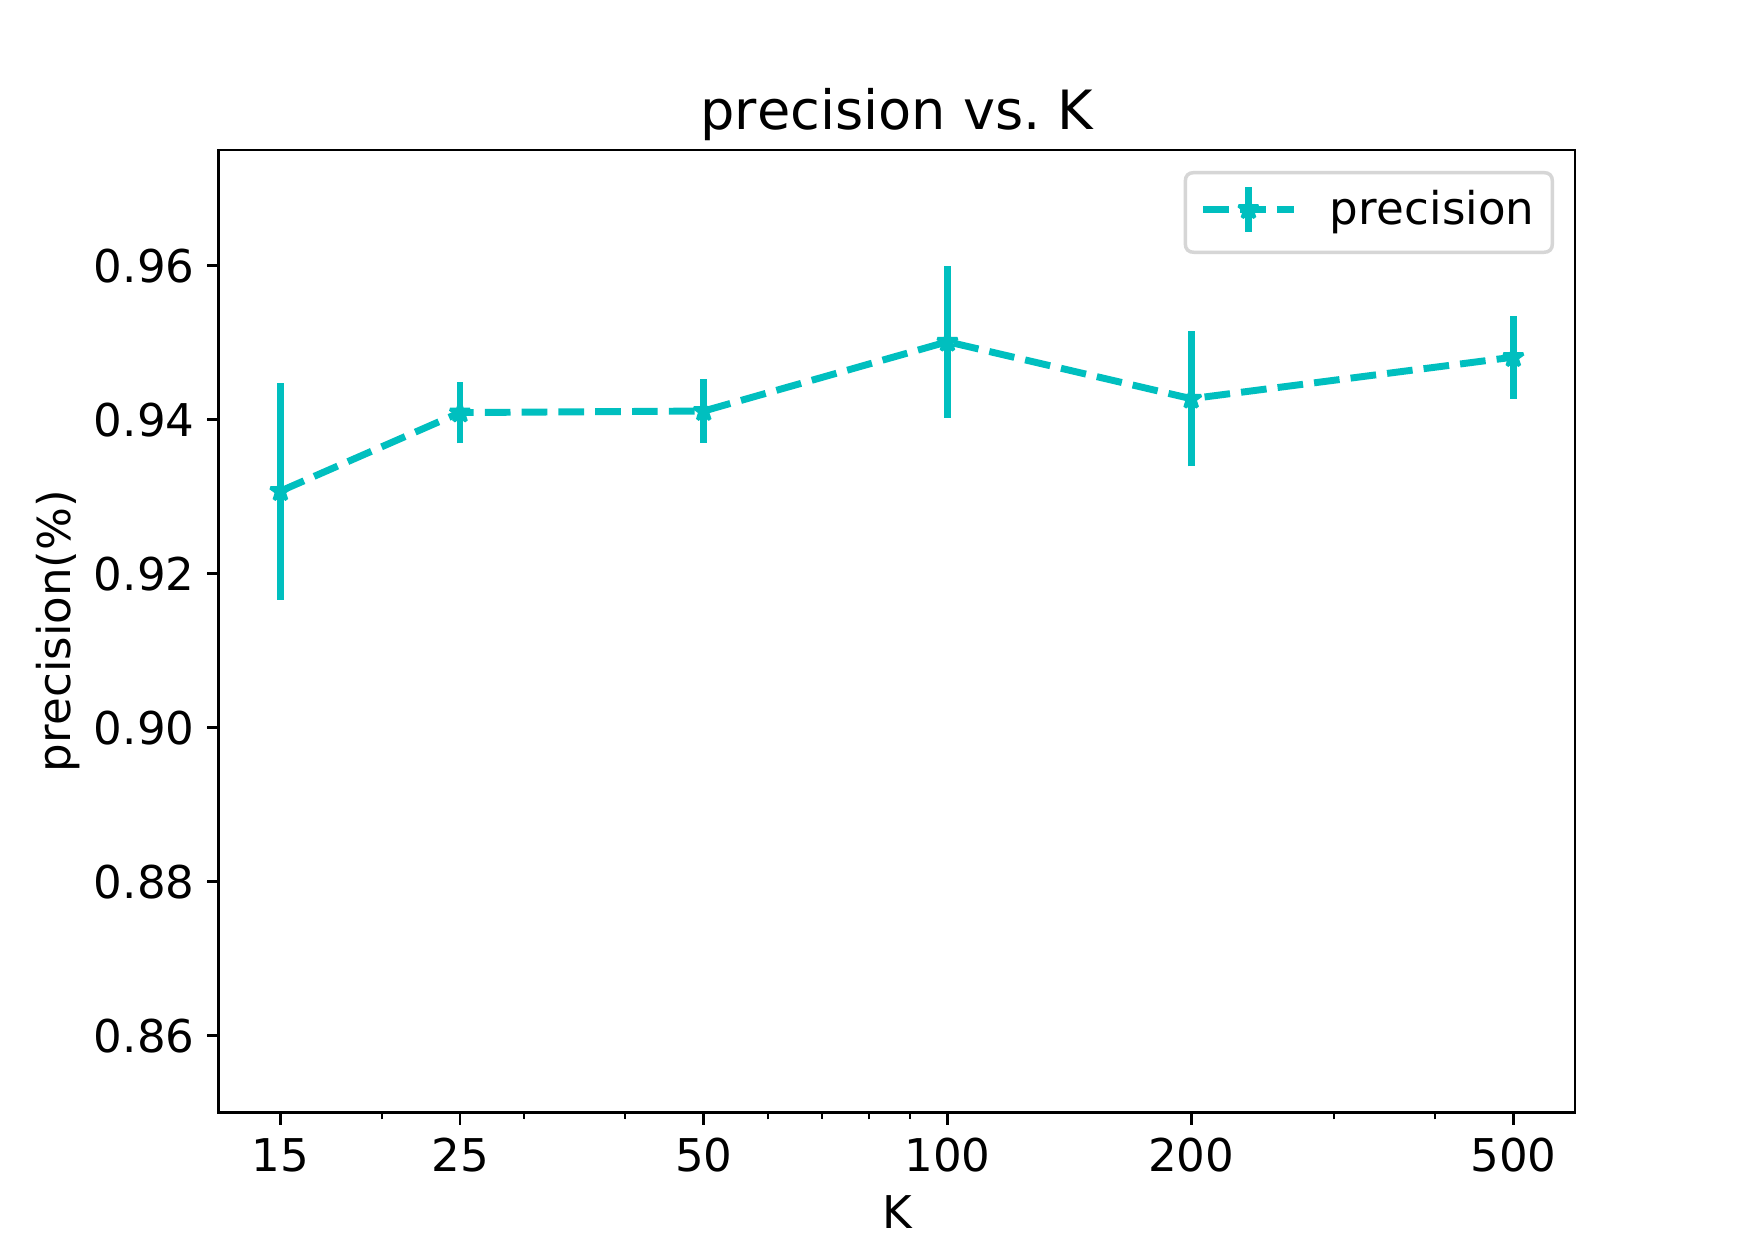}
%     \includegraphics[width=0.45\textwidth]{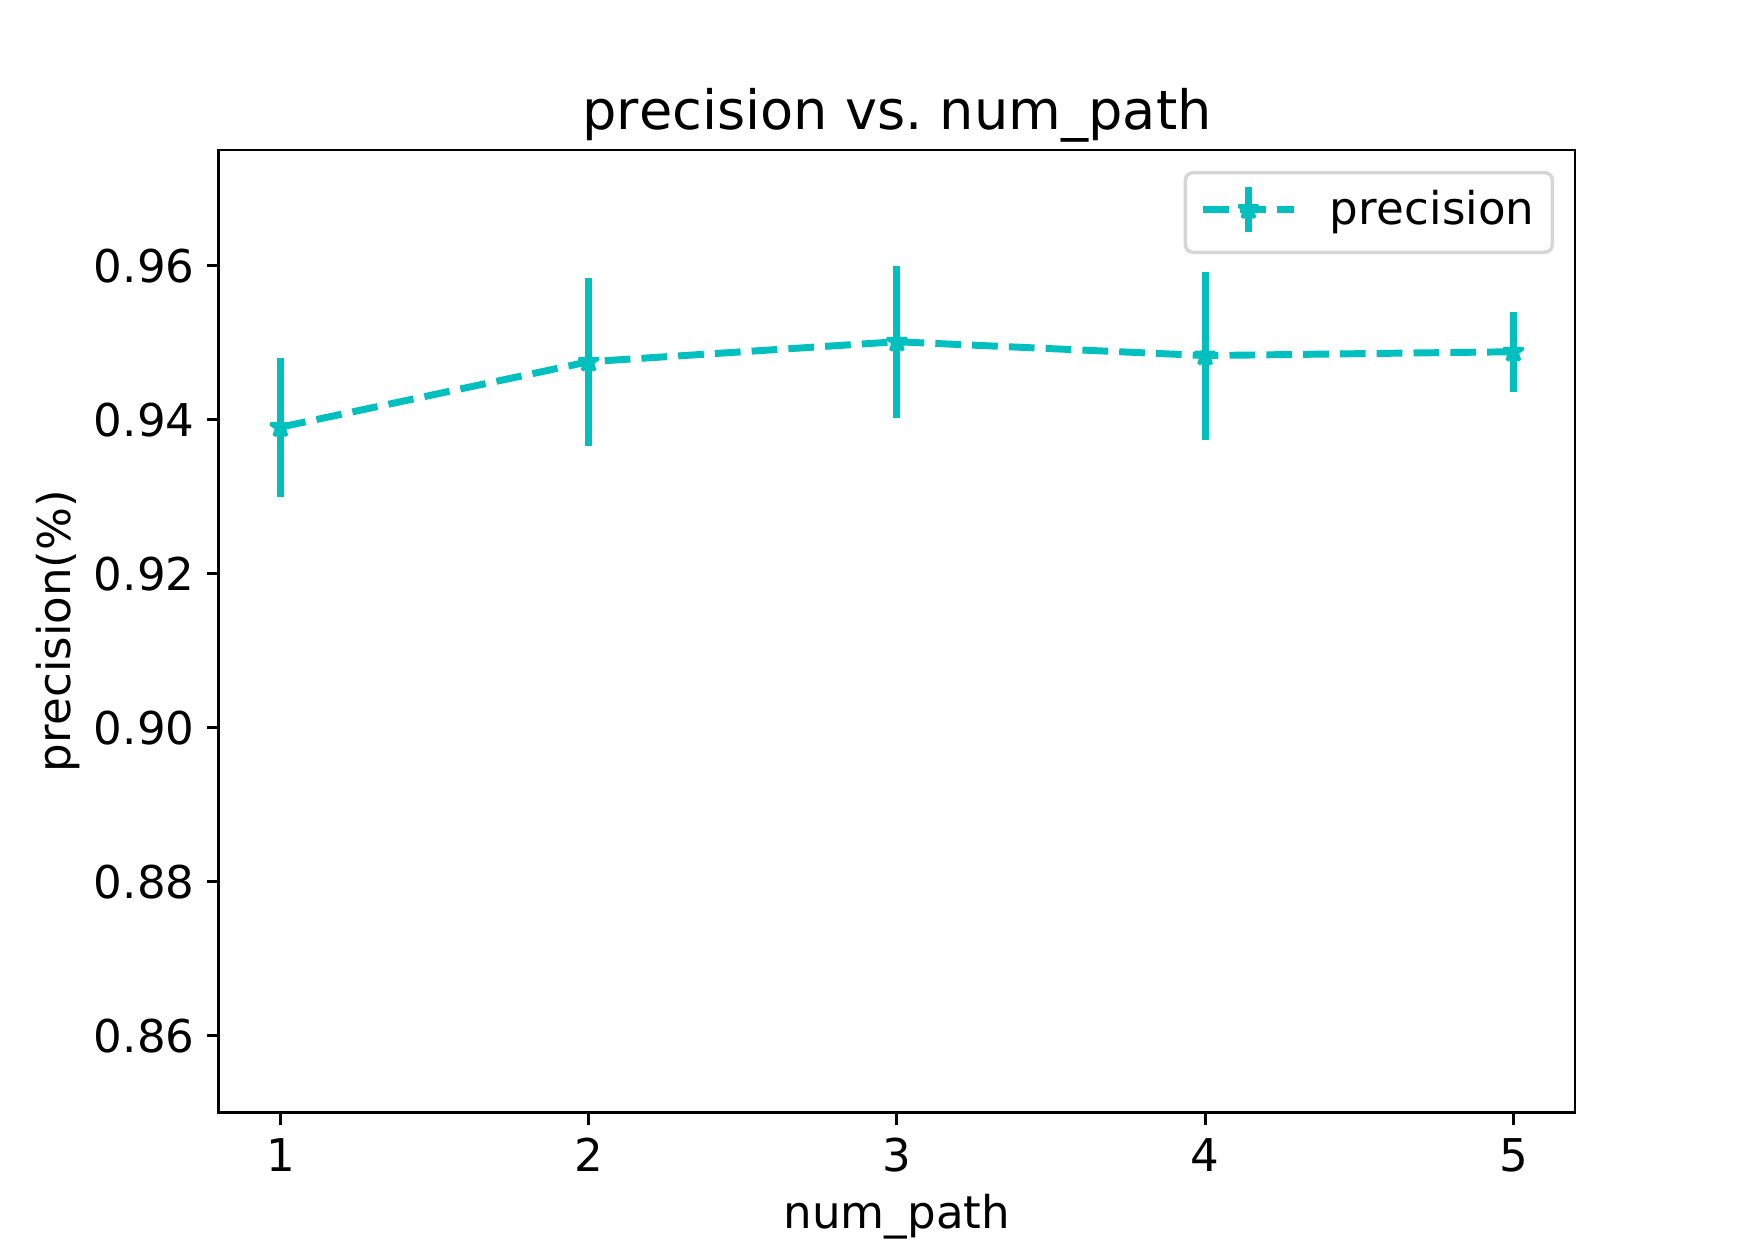}
%     \includegraphics[width=0.45\textwidth]{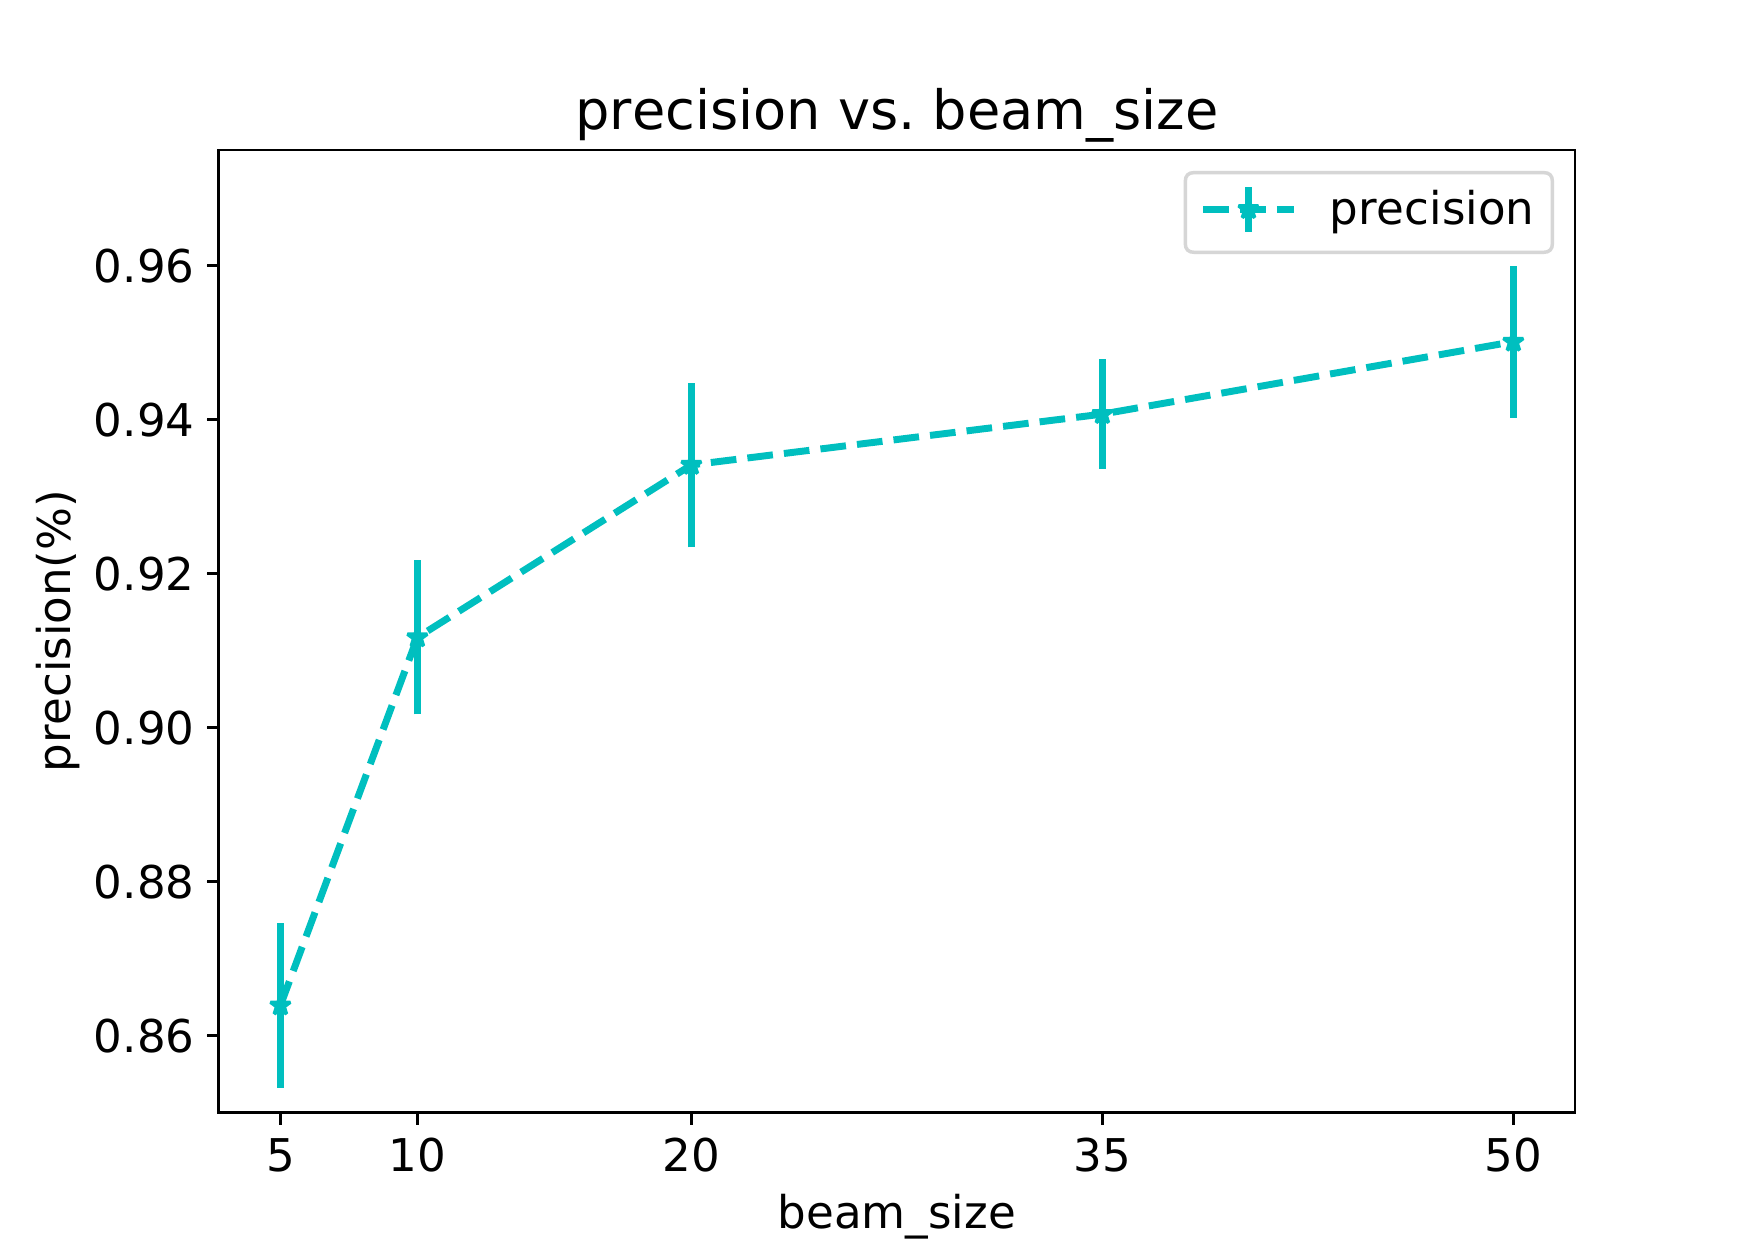}
%     \includegraphics[width=0.45\textwidth]{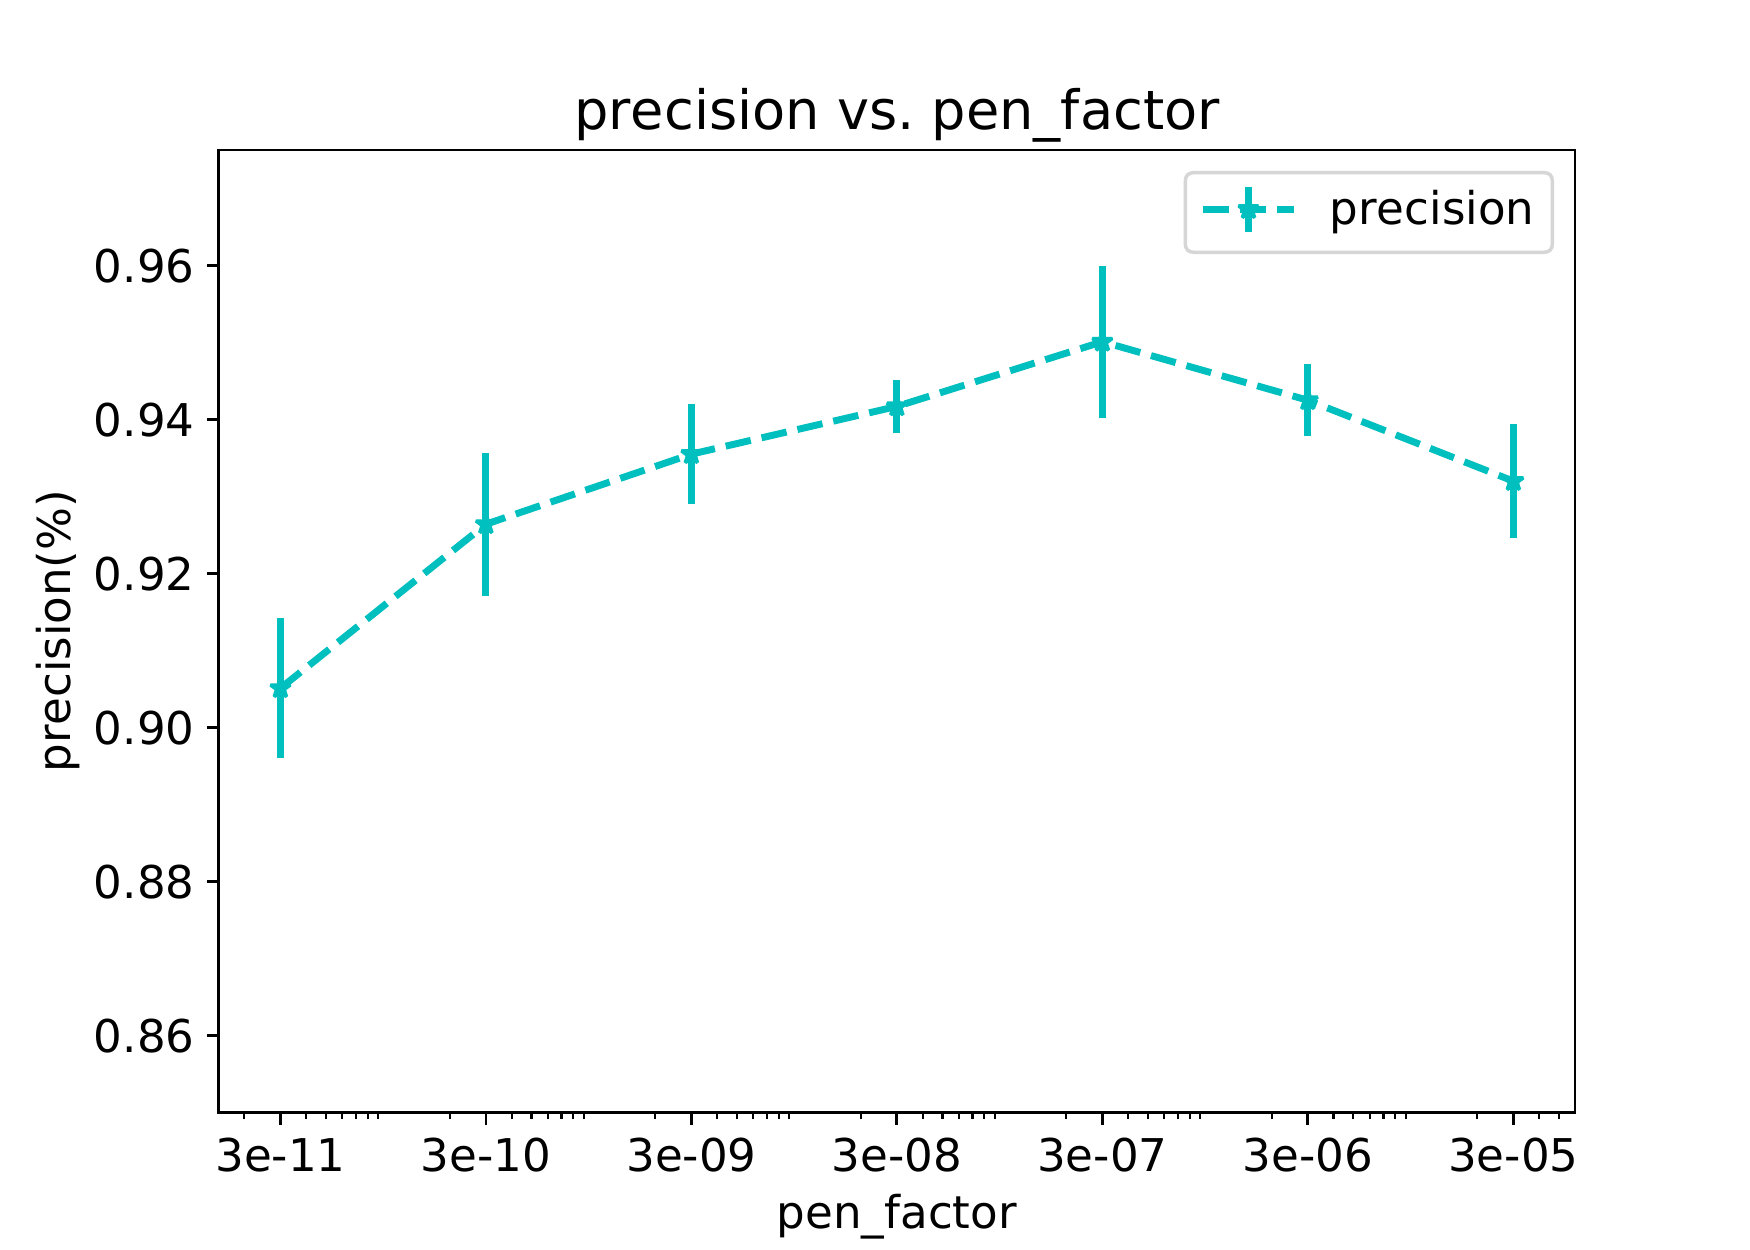}
%     \caption{Relationship between precision@200 in Amazon Books experiment and model width $K$, number of paths $J$, beam size $B$ and penalty factor $\alpha$, respectively.}
%     \label{fig:hyperparameters_2}
% \end{figure}

% \begin{figure}[H]
%     \centering
%     \includegraphics[width=0.45\textwidth]{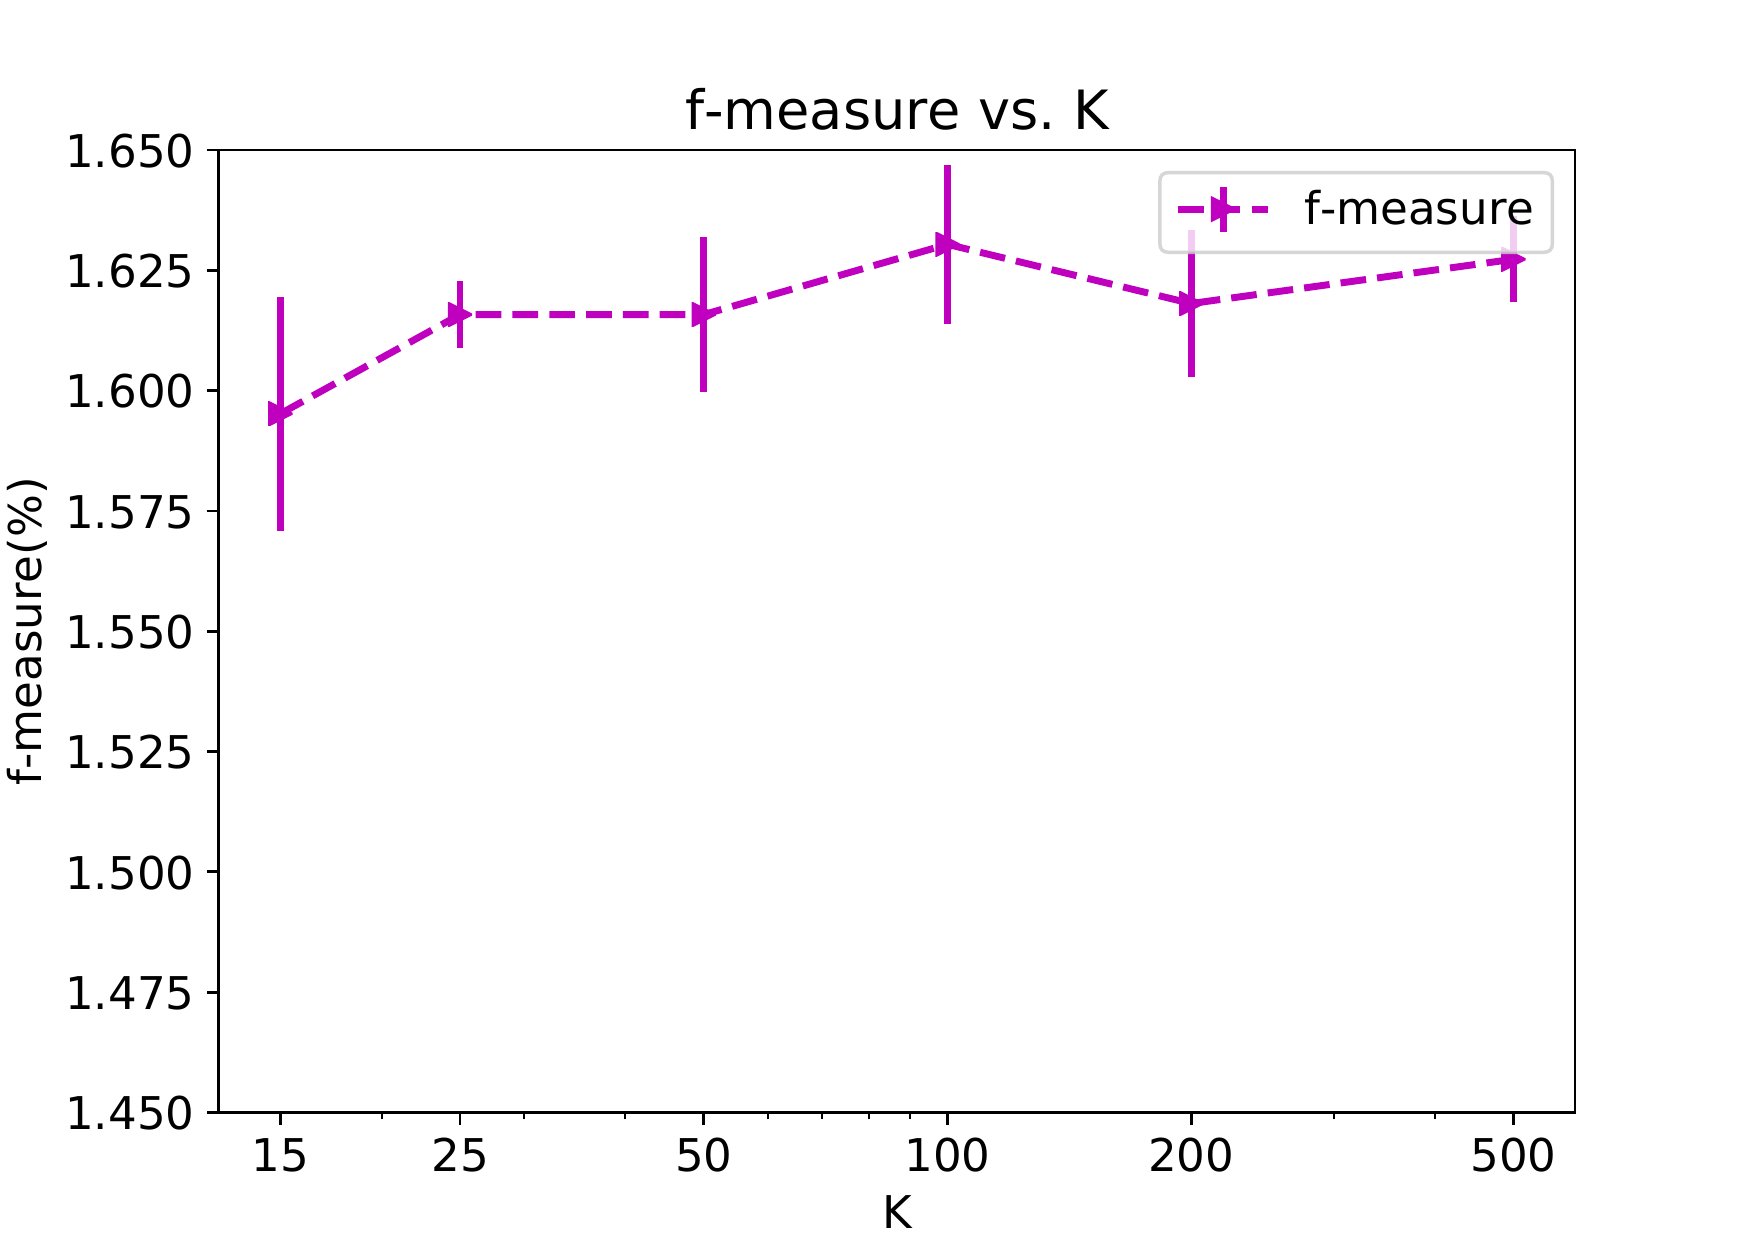}
%     \includegraphics[width=0.45\textwidth]{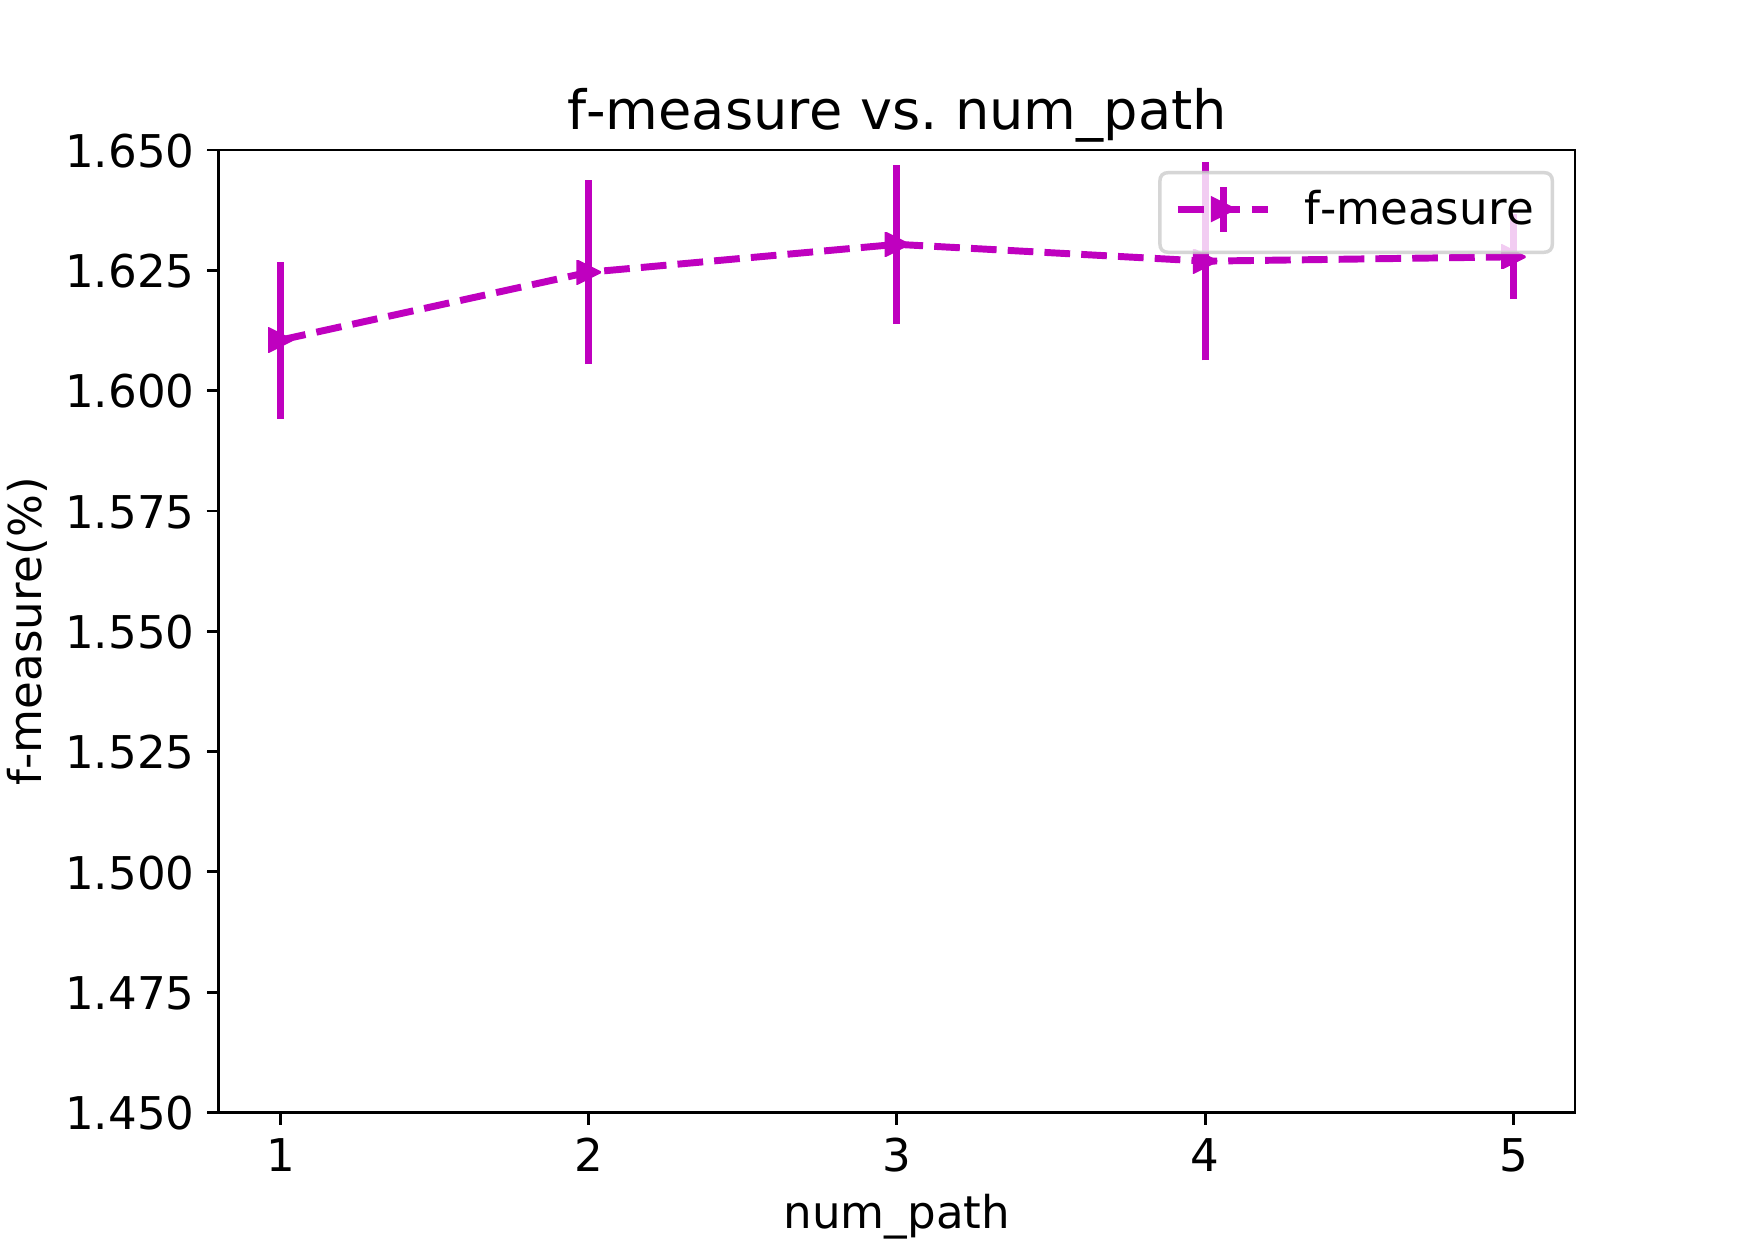}
%     \includegraphics[width=0.45\textwidth]{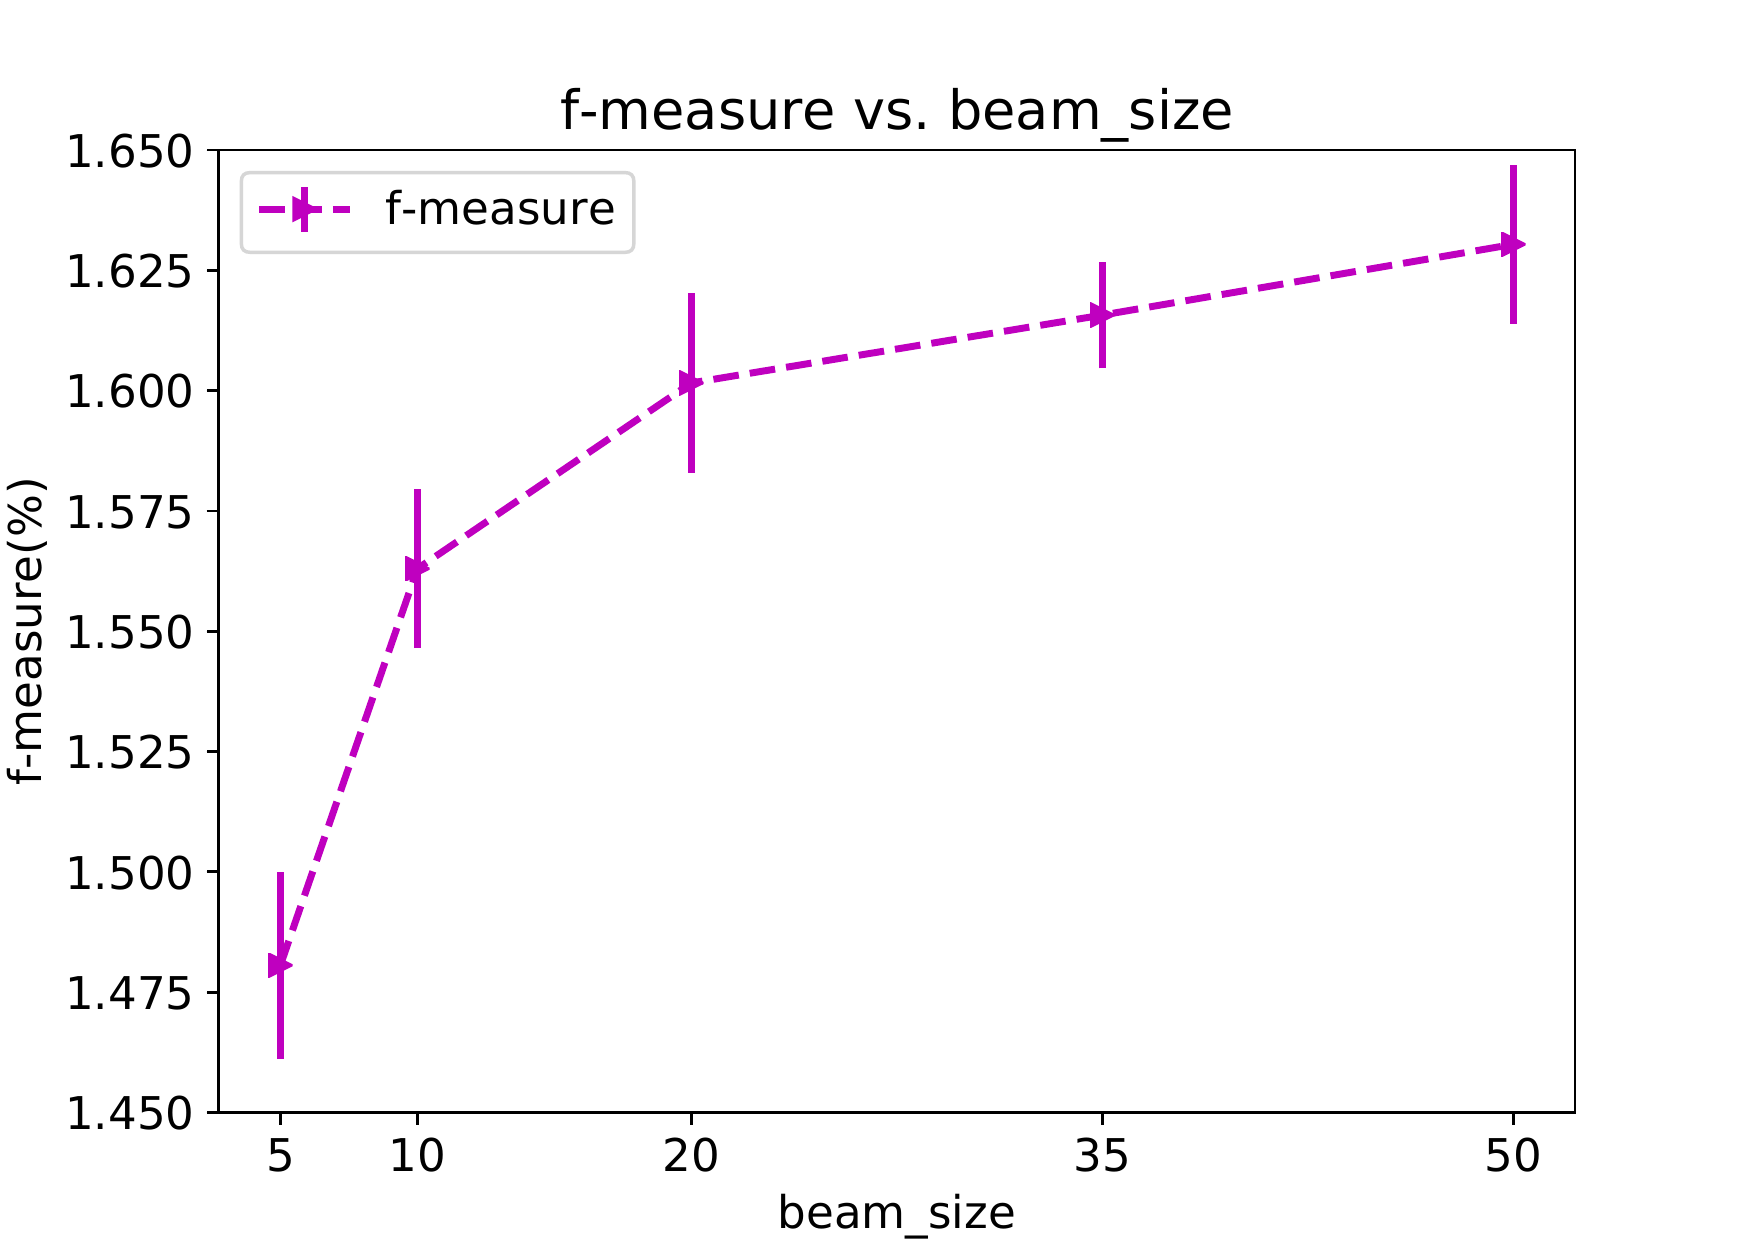}
%     \includegraphics[width=0.45\textwidth]{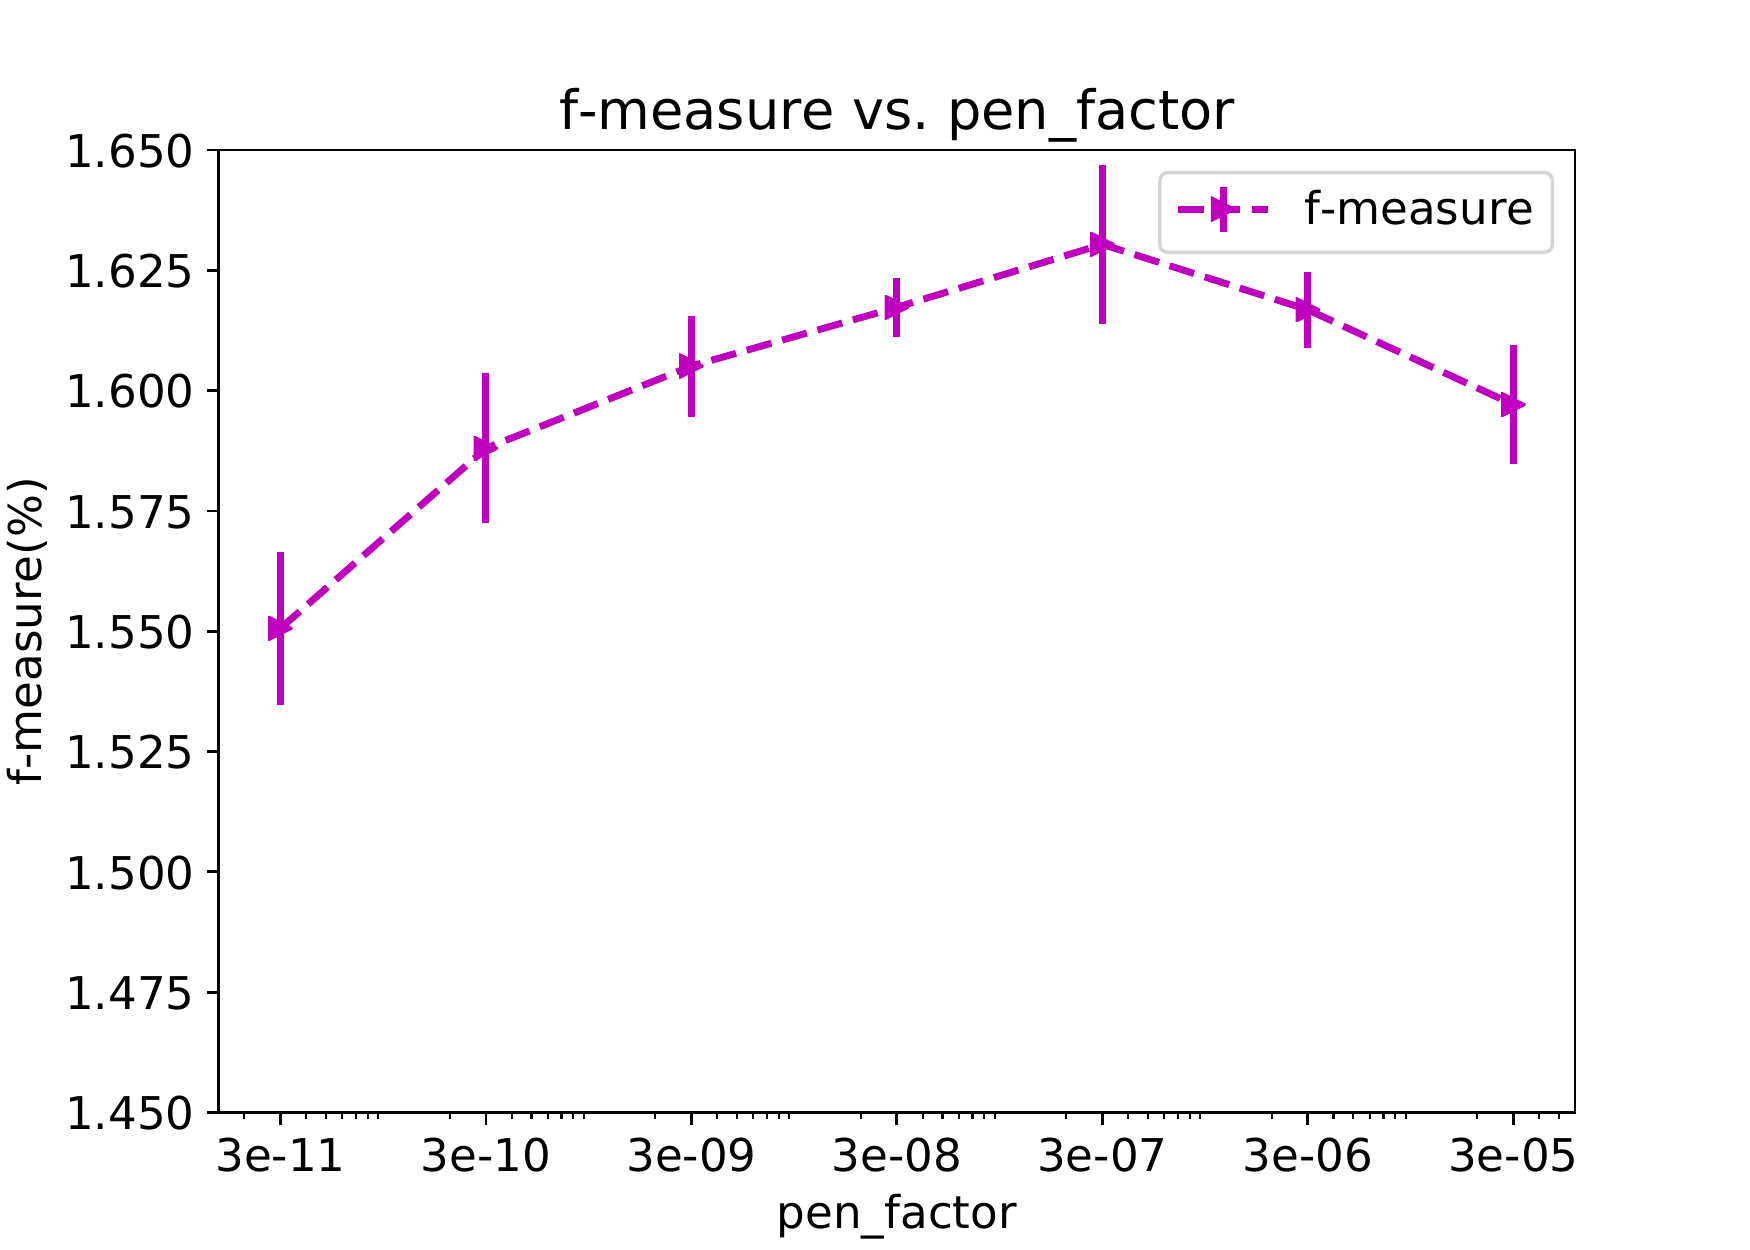}
%     \caption{Relationship between F-measure@200 in Amazon Books experiment and model width $K$, number of paths $J$, beam size $B$ and penalty factor $\alpha$, respectively.}
%     \label{fig:hyperparameters_3}
% \end{figure}

\newpage
